# Supplementary material for: Axionic quantum criticality of generalized Weyl semimetals
Source: arXiv:2412.09609 ancillary file (2025-03-31)
Supplement: Supplementary file 1 [file Axionic_criticality-SM.pdf]

# Supplemental Material:
# Axionic quantum criticality of generalized Weyl semimetals

Gabriel Malavé[1], Rodrigo Soto-Garrido[1], Vladimir Juričić[2], and Bitan Roy[3]

[1]Instituto de Física, Pontificia Universidad Católica de Chile, Santiago, 7820436, Chile
[2]Departamento de Física, Universidad Técnica Federico Santa María, Casilla 110, Valparaíso, Chile
[3]Department of Physics, Lehigh University, Bethlehem, Pennsylvania, 18015, USA

**Abstract**

This Supplemental Material contains: Details of the model of a generalized Weyl semimetal [Sec. S1]; The calculation of the resummed (dressed) bosonic propagator [Sec. S2]; Details of the derivation of the renormalization-group flow equations [Sec. S3]; The calculation of the one-loop counterterms [Sec. S4]; The calculation of RG fixed points, anomalous dimensions and critical exponents [Sec. S5].

## Contents

**1 The model** **1**

**2 Resummed boson propagator** **3**
2.1 Limiting cases . . . . . 7

**3 Derivation of the RG equations** **8**

**4 One-loop counter-terms** **9**
4.1 Boson self-energy . . . . . 9
4.2 Fermion self-energy . . . . . 9
4.3 Vertex correction . . . . . 12

**5 RG fixed points and critical exponents** **12**

## 1 The model

The effective single-particle Hamiltonian describing a $d$-dimensional non-interacting nodal-point semimetal with linear dispersion along $d_L$ directions and dispersion with finite curvature along $d_M$ directions is given by

$$H_0\left(k_i\right) = \sum_{l=1}^{d_L} \Gamma_l k_l + \sum_{r=1}^{d_M} \Gamma_{d_L+r} \varepsilon_r \left(k_{d_L+1}, \ldots, k_d\right) \tag{1}$$

where $k_i$ are the components of momentum, $\{\Gamma_i\}$ are a set of mutually anticommuting Hermitian matrices of dimension $4N$, satisfying $\{\Gamma_j, \Gamma_k\} = \delta_{jk}$, $\varepsilon_r$ are non-linear functions of their arguments and $d = d_L + d_M$. Short-ranged Hubbard-like interactions can trigger a symmetry breaking phase by generating a mass term $\sum_{a=1}^{N_b} M_a \Upsilon_a$, where $\{\Upsilon_a\}$ is another set of anticommuting matrices, satisfying $\{\Upsilon_j, \Upsilon_k\} = 2\delta_{jk}$, and $N_b$ is the number of order parameter components. Such an ordering leads to a fully gapped state, since $\{\Gamma_j, \Upsilon_k\} = 0$, where the magnitude of $\boldsymbol{M}$ determines the condensation energy gain. Here we focus on the quantum critical point (QCP) controlling such a transition.

Near the QCP the relevant degrees of freedom are gapless nodal fermions and bosonic order parameter fluctuations, which are coupled via a Yukawa interaction [1]. The effective action can be written as

$$
\begin{aligned}
S = &\sum_{n=1}^{N_f} \int_k \psi^\dagger_{n,k} G_0^{-1}(k) \psi_{n,k} + \frac{1}{2}\sum_{a=1}^{N_b} \int_q D_0^{-1}(q) \phi^a_{-q}\phi^a_q + \frac{g_0}{\sqrt{N_f}} \sum_{n=1}^{N_f}\sum_{a=1}^{N_b} \int_{k,q} \phi^a_q \left( \psi^\dagger_{n,k+q} \Upsilon_a \psi_{n,k} \right) \\
&+ \frac{u_0}{2} \sum_{a=1}^{N_b}\sum_{b=1}^{N_b} \int_{k,q,q'} \phi^a_{-q}\phi^a_{q+q'}\ \phi^b_{-k}\phi^b_{k-q'},
\end{aligned} \tag{2}
$$

where $k = (k_0, k_1, ..., k_d)$, with $k_0$ being the Euclidean frequency. The bare fermionic and bosonic propagators are

$$
G_0(k) = \left[ik_0 + H_0(k_1, ..., k_d)\right]^{-1} \tag{3}
$$

$$
D_0(q) = \left[ c^2 \left( q_0^2 + \sum_{l=1}^{d_L} q_l^2 \right) + \sum_{n=d_L+1}^{d_M} q_n^2 + |\vec{M}|^2 \right]^{-1}, \tag{4}
$$

respectively. The parameter $c$ encodes an anisotropy of the bosonic dynamics, stemming from the anisotropic fermionic disperion.

It is convenient to define a $(d_L+1)$-dimesional frequency-momentum vector $\boldsymbol{k} \equiv (k_0, k_1, ..., k_{d_L})$ and a $d_M$-dimensional momentum $\boldsymbol{K} \equiv (k_{d_L+1}, ..., k_d)$. The noninteracting part of this action is invariant under the scaling $[\boldsymbol{K}] = 1$ and $[\boldsymbol{k}] = z_{\boldsymbol{k}}$, implying that:

- $[G_0^{-1}] = [\boldsymbol{k}] = z_{\boldsymbol{k}}$. The fermionic part of the action then yields $z_{\boldsymbol{k}}(d_L+1) + d_M + z_{\boldsymbol{k}} + 2[\psi] = 0$, such that

$$
[\psi] = -\frac{z_{\boldsymbol{k}}(d_L+2) + d_M}{2}. \tag{5}
$$

- $[D_0^{-1}] = 2$, such that $[c] = 1 - z_{\boldsymbol{k}}$ and $[M] = 1$. The bosonic part of the action then yields $z_{\boldsymbol{k}}(d_L+1) + d_M + 2 + 2[\phi] = 0$, such that

$$
[\phi] = -1 - \frac{z_{\boldsymbol{k}}(d_L+1) + d_M}{2}. \tag{6}
$$

- From the Yukawa term we find $[g_0] + 2(z_{\boldsymbol{k}}(d_L+1) + d_M) + [\phi] + 2[\psi] = 0$, such that

$$
[g_0] = -2(z_{\boldsymbol{k}}(d_L+1) + d_M) + 1 + \frac{z_{\boldsymbol{k}}(d_L+1) + d_M}{2} + z_{\boldsymbol{k}}(d_L+2) + d_M = 1 - \frac{z_{\boldsymbol{k}}(d_L-1) + d_M}{2}. \tag{7}
$$

- For the $\phi^4$ term we have $[u_0] + 3(z_{\boldsymbol{k}}(d_L+1) + d_M) + 4[\phi] = 0$, such that

$$
[u_0] = -3(z_{\boldsymbol{k}}(d_L+1) + d_M) + 4 + 2(z_{\boldsymbol{k}}(d_L+1) + d_M) = 4 - z_{\boldsymbol{k}}(d_L+1) - d_M. \tag{8}
$$

For a power $n$ band dispersion, the action is invariant under the tree-level scaling upon setting $z_{\boldsymbol{k}} = n$ at the non-interacting fixed point. The Yukawa coupling is then marginal on the line $z_{\boldsymbol{k}}(d_L-1) + d_M = 2$, which always passes through $(d_L, d_M) = (1, 2)$, representing the QCP that we analyze here. On this line the $\phi^4$ term is then irrelevant for $n > 1$. Interacting fixed points where the Yukawa coupling is dimensionful can be reached by independently tuning the deviations $\epsilon_L = \bar{d}_L - d_L$ and $\epsilon_M = \bar{d}_M - d_M$, where $z_{\boldsymbol{k}}(\bar{d}_L - 1) + \bar{d}_M = 2$. This is accomplished through dimensional regularization and the RG equations, a procedure we carry out here.

We now focus on a Hamiltonian that captures the low-energy physics of a generalized Weyl semimetal (WSM) with the two nodal points characterized by the monopole charges $\pm n$,

$$H_n(k_x, k_y, k_z) = \alpha_n k_\perp^n \left[\Gamma_1 \cos(n\phi_k) + \Gamma_2 \sin(n\phi_k)\right] + \Gamma_3 v_z k_z, \tag{9}$$

$$\Gamma_1 = \tau_0 \otimes \sigma_1, \quad \Gamma_2 = \tau_0 \otimes \sigma_2, \quad \Gamma_3 = \tau_3 \otimes \sigma_3, \tag{10}$$

$$k_\perp^2 = k_x^2 + k_y^2, \quad \phi_k = \tan^{-1}(k_y/k_x). \tag{11}$$

For suficiently strong interactions, this WSM can undergo a quantum phase transition into a translational symmetry breaking axion insulator (AI) [2]. In proximity to the axionic charge-density wave ordering, $N_b = 2$ and correspondingly $\Upsilon_1 \equiv \Gamma_4 = \tau_1 \otimes \sigma_3$ and $\Upsilon_2 \equiv \Gamma_5 = \tau_2 \otimes \sigma_3$. The bare fermionic propagator is

$$G_0(k) = [i\omega + H_n(k_x, k_y, k_z)]^{-1}, \tag{12}$$

where $k \equiv (\omega, k_x, k_y, k_z)$, with $\omega$ being the Euclidean frequency. The corresponding momentum 2-vectors are $\boldsymbol{k} \equiv (\omega, k_z)$ and $\boldsymbol{K} \equiv (k_x, k_y)$.

## 2 Resummed boson propagator

In this section we present the calculational details of the dressed boson propagator $D(q)$ close to $d = 3$ spatial dimensions, following the procedure outlined in Ref. [1] and the main manuscript. We consider the polarization bubble

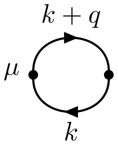


$$\nu = i\,\Pi_{\mu\nu}(q) = -ig^2 \int \mathrm{d}k\, \mathrm{Tr}\left\{G_0(k+q)\ \tau_\mu \otimes \sigma_0\ G_0(k)\ \tau_\nu \otimes \sigma_0\right\}. \tag{13}$$

The calculation of $\Pi_{\mu\nu}(q)$ consists of generalizing the dimension of the $\boldsymbol{k}$-space to be $d = 2(1 - \epsilon_b)$ while imposing a hard UV cutoff such that $|\boldsymbol{K}| \leq \Lambda$. Given that all the $\Gamma_i$ are mutually anticommuting, the trace enforces $\Pi_{\mu\nu}(q) = \Pi(q)\delta_{\mu\nu}$ and we only need to consider the diagonal part $\mu = \nu$.

Since the vertex matrices $\tau_\mu \otimes \sigma_0$ anticommute with $H_{\mathrm{nW}}$, we first make the following replacement:

$$\begin{aligned} G_0(k+q)\ \tau_\mu \otimes \sigma_0\ G_0(k)\ \tau_\nu \otimes \sigma_0 &= \frac{-i(\omega + q_0) + H_n(k+q)}{(\omega+q_0)^2 + H_n^2(k+q)}\ \tau_\mu \otimes \sigma_0\ \frac{-i\omega + H_n(k)}{\omega^2 + H_n^2(k)}\ \tau_\nu \otimes \sigma_0 \\ &\to -\frac{-i(\omega + q_0) + H_n(k+q)}{(\omega+q_0)^2 + H_n^2(k+q)}\ \frac{i\omega + H_n(k)}{\omega^2 + H_n^2(k)}\ \delta_{\mu\nu}. \end{aligned} \tag{14}$$

We now absorb the constants $\alpha_n$ and $v_z$ in the corresponding momenta, and the form of Eq. (9) implies

$$H_n^2(k) = k_z^2 + (|\boldsymbol{K}|^n)^2 \tag{15}$$

$$H_n^2(k+q) = (k_z + q_z)^2 + (|\boldsymbol{K} + \boldsymbol{Q}|^n)^2. \tag{16}$$

Defining the angles $\phi$ and $\phi'$ by

$$k_x = |\boldsymbol{K}| \cos\phi, \quad k_y = |\boldsymbol{K}| \sin\phi, \tag{17}$$

$$(k_x + q_x) = |\boldsymbol{K} + \boldsymbol{Q}| \cos\phi', \quad (k_y + q_y) = |\boldsymbol{K} + \boldsymbol{Q}| \sin\phi', \tag{18}$$

and after taking the trace, we find

$$\begin{aligned}&\mathrm{Tr}\left\{[-i(\omega+q_0)+H_n(k+q)][i\omega+H_n(k)]\right\}\\&\quad=4N\left\{\boldsymbol{k}\cdot(\boldsymbol{k}+\boldsymbol{q})+|\boldsymbol{K}+\boldsymbol{Q}|^n|\boldsymbol{K}|^n(\cos n\phi'\cos n\phi+\sin n\phi'\sin n\phi)\right\}\\&\quad=4N\left\{\boldsymbol{k}\cdot(\boldsymbol{k}+\boldsymbol{q})+|\boldsymbol{K}+\boldsymbol{Q}|^n|\boldsymbol{K}|^n\cos[n(\phi-\phi')]\right\}.\end{aligned}\tag{19}$$

Then we combine the denumerators by means of Feynman parametrization:

$$\frac{1}{(\boldsymbol{k}+\boldsymbol{q})^2+\left(|\boldsymbol{K}+\boldsymbol{Q}|^n\right)^2}\frac{1}{\boldsymbol{k}^2+\left(|\boldsymbol{K}|^n\right)^2}=\int_0^1 dx\frac{1}{\left[\boldsymbol{k}^2+2x\boldsymbol{k}\cdot\boldsymbol{q}+x\boldsymbol{q}^2+x\left(|\boldsymbol{K}+\boldsymbol{Q}|^n\right)^2+(1-x)\left(|\boldsymbol{K}|^n\right)^2\right]^2}\tag{20}$$

$$=\int_0^1 dx\frac{1}{\left(\boldsymbol{k'}^2+M\right)^2},\tag{21}$$

where $\boldsymbol{k'}=\boldsymbol{k}+x\boldsymbol{q}$ and $M=x(1-x)\boldsymbol{q}^2+x\left(|\boldsymbol{K}+\boldsymbol{Q}|^n\right)^2+(1-x)\left(|\boldsymbol{K}|^n\right)^2$, and $x$ is the Feynman parameter. Collecting the obtained terms in Eq. (13):

$$\Pi(q)=4Ng^2\int_0^1 dx\int \mathrm{d}\boldsymbol{K}\int\frac{d^d\boldsymbol{k'}}{(2\pi)^d}\frac{\boldsymbol{k'}^2-x(1-x)\boldsymbol{q}^2+|\boldsymbol{K}|^n|\boldsymbol{K}+\boldsymbol{Q}|^n\cos[n(\phi-\phi')]}{\left(\boldsymbol{k'}^2+M\right)^2},\tag{22}$$

where the terms linear in $\boldsymbol{k'}$ have been neglected since they vanish by symmetry upon integration. The integral over $\boldsymbol{k'}$ can be performed with the dimensional regularization formulae [3]:

$$\int\frac{d^d\ell}{(2\pi)^d}\frac{1}{\left(\ell^2+\Delta\right)^n}=\frac{1}{(4\pi)^{d/2}}\frac{\Gamma\left(n-\frac{d}{2}\right)}{\Gamma(n)}\left(\frac{1}{\Delta}\right)^{n-\frac{d}{2}}\tag{23}$$

$$\int\frac{d^d\ell}{(2\pi)^d}\frac{\ell^2}{\left(\ell^2+\Delta\right)^n}=\frac{1}{(4\pi)^{d/2}}\frac{d}{2}\frac{\Gamma\left(n-\frac{d}{2}-1\right)}{\Gamma(n)}\left(\frac{1}{\Delta}\right)^{n-\frac{d}{2}-1}\tag{24}$$

$$\Gamma(x)=\frac{1}{x}-\gamma+\mathcal{O}(x),\tag{25}$$

near $x=0$ where $\gamma\approx 0.5772$ is the Euler-Mascheroni constant. This yields

$$\begin{aligned}&\int\frac{d^d\boldsymbol{k'}}{(2\pi)^d}\frac{\boldsymbol{k'}^2-x(1-x)\boldsymbol{q}^2+|\boldsymbol{K}+\boldsymbol{Q}|^n|\boldsymbol{K}|^n\cos[n(\phi-\phi')]}{\left(\boldsymbol{k'}^2+M\right)^2}\\&\quad=\frac{1}{(4\pi)^{d/2}}\left\{\frac{d}{2}\Gamma(1-d/2)\left(\frac{1}{M}\right)^{1-d/2}+\left[x(x-1)\boldsymbol{q}^2+|\boldsymbol{K}|^n|\boldsymbol{K}+\boldsymbol{Q}|^n\cos[n(\phi-\phi')]\right]\Gamma(2-d/2)\left(\frac{1}{M}\right)^{2-d/2}\right\}\\&\quad\underset{\epsilon_b\to 0}{\to}\frac{1}{(4\pi)}\left\{\epsilon_b^{-1}-\gamma+\ln 4\pi-1-\ln M+\frac{x(x-1)\boldsymbol{q}^2+|\boldsymbol{K}|^n|\boldsymbol{K}+\boldsymbol{Q}|^n\cos[n(\phi-\phi')]}{M}\right\}.\end{aligned}\tag{26}$$

Neglecting the constant finite terms, we obtain

$$\Pi(q)=N\frac{g^2}{\pi}\int_0^1 dx\int\mathrm{d}\boldsymbol{K}\left\{\epsilon_b^{-1}-\ln M+\frac{x(x-1)\boldsymbol{q}^2+|\boldsymbol{K}|^n|\boldsymbol{K}+\boldsymbol{Q}|^n\cos[n(\phi-\phi')]}{M}\right\}.\tag{27}$$

To deal with the cosine, we consider the vectors and angles shown in Fig. 1, which are related by

$$|\boldsymbol{K}+\boldsymbol{Q}||\boldsymbol{K}|\cos[(\phi-\phi')]=\boldsymbol{K}\cdot(\boldsymbol{K}+\boldsymbol{Q})=|\boldsymbol{K}|^2+|\boldsymbol{Q}||\boldsymbol{K}|\cos\theta,\tag{28}$$

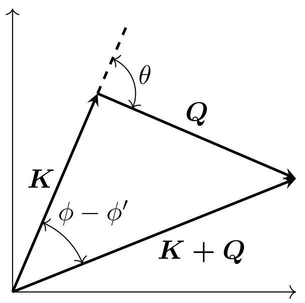


Figure 1: Relevant vectors and angles involved in the calculation of $\Pi(q)$, given by Eq. (13).

where $\theta$ is the angle between $\boldsymbol{K}$ and $\boldsymbol{Q}$.

Since the function $\cos(nx)$ can be written in terms of Chebyshev polynomials as $\cos(nx) = T_n(\cos x)$, the last term in the numerator of Eq. (27) can be written as a polynomial of degree $2n$ in $|\boldsymbol{K}|$ and degree $n$ in $\cos\theta$. In the scaling given by the definitions $|\boldsymbol{K}| = z^{1/2}|\boldsymbol{q}|^{1/n}$, $|\boldsymbol{Q}| = \widetilde{Q}|\boldsymbol{q}|^{1/n}$ and $\Lambda = \widetilde{\Lambda}|\boldsymbol{q}|^{1/n}$, we will always have

$$|\boldsymbol{K}|^n|\boldsymbol{K}+\boldsymbol{Q}|^n\cos[n(\phi-\phi')] = |\boldsymbol{q}|^2\left(z^n + P_n(z,\theta,\widetilde{Q})\right), \tag{29}$$

where $P_n(z,\theta,\widetilde{Q})$ is a polynomial of degree $(2n-1)/2$ in $z$ and of degree $n$ in $\cos\theta$, and we have used the fact that the coefficients of $T_n(x)$ always sum to 1. Under this scaling we also have

$$M = |\boldsymbol{q}|^2\left[x(1-x) + x\left(z+\tilde{Q}^2+2\sqrt{z}\tilde{Q}\cos\theta\right)^n + (1-x)z^n\right], \tag{30}$$

$$\int_{|\boldsymbol{K}|<\Lambda} \mathrm{d}\boldsymbol{K} \to \frac{|\boldsymbol{q}|^{2/n}}{2(2\pi)}\int_0^{2\pi}\frac{d\theta}{2\pi}\int_0^{\widetilde{\Lambda}^2} dz. \tag{31}$$

Defining $\mathcal{N} = \left(z+\widetilde{Q}^2+2\sqrt{z}\widetilde{Q}\cos\theta\right)$, we can write:

$$\Pi(q) = N\frac{g^2|\boldsymbol{q}|^{2/n}}{(2\pi)^2}\int_0^{2\pi}\frac{d\theta}{2\pi}\int_0^{\widetilde{\Lambda}^2}dz\int_0^1 dx \tag{32}$$

$$\left\{\left(\epsilon_b^{-1}-\ln|\boldsymbol{q}|^2\right) - \ln\left[x(1-x)+x\mathcal{N}^n+(1-x)z^n\right] + \frac{x(x-1)+z^n+P_n(z,\theta,\widetilde{Q})}{x(1-x)+x\mathcal{N}^n+(1-x)z^n}\right\}. \tag{33}$$

Integrating the logarithm by parts:

$$\begin{aligned}\Pi(q) = N\frac{g^2|\boldsymbol{q}|^{2/n}}{(2\pi)^2}\int_0^{2\pi}\frac{d\theta}{2\pi}\int_0^{\widetilde{\Lambda}^2}dz\,&\left\{\left(\epsilon_b^{-1}-\ln|\boldsymbol{q}|^2\right) - x\ln\left[x(1-x)+x\mathcal{N}^n+(1-x)z^n\right]\Big|_0^1\right. \\ &\left.+\int_0^1 dx\frac{x(1-2x+\mathcal{N}^n-z^n)}{x(1-x)+x\mathcal{N}^n+(1-x)z^n} + \int_0^1 dx\frac{x(x-1)+z^n+P_n(z,\theta,\widetilde{Q})}{x(1-x)+x\mathcal{N}^n+(1-x)z^n}\right\} \\ = N\frac{g^2|\boldsymbol{q}|^{2/n}}{(2\pi)^2}\int_0^{2\pi}\frac{d\theta}{2\pi}\int_0^{\widetilde{\Lambda}^2}dz\,&\left\{\left(\epsilon_b^{-1}-\ln|\boldsymbol{q}|^2\right) - \ln\mathcal{N}^n + \int_0^1 dx\frac{-x^2+x(\mathcal{N}^n-z^n)+z^n+P_n(z,\theta,\widetilde{Q})}{-x^2+x(1+\mathcal{N}^n-z^n)+z^n}\right\} \\ = N\frac{g^2|\boldsymbol{q}|^{2/n}}{(2\pi)^2}\int_0^{2\pi}\frac{d\theta}{2\pi}\int_0^{\widetilde{\Lambda}^2}dz\,&\left\{\left(\epsilon_b^{-1}-\ln|\boldsymbol{q}|^2\right) \underbrace{-\ln\mathcal{N}^n + \int_0^1 dx\frac{x-P_n(z,\theta,\widetilde{Q})}{x^2-x\left(1+\mathcal{N}^n-z^n\right)-z^n}}_{h_n(z,\theta,\widetilde{Q})} + 1\right\}.\end{aligned} \tag{34, 35}$$

After integrating over the Feynman parameter $x$ we find

$$h_n(z,\theta,\widetilde{Q}) = -\ln z^n + \frac{\left(2P_n(z,\theta,\widetilde{Q}) - \mathcal{N}^n + z^n - 1\right)\coth^{-1}\left(\frac{\mathcal{N}^n+z^n+1}{\sqrt{\mathcal{N}^{2n}-2\mathcal{N}^n(z^n-1)+(z^n+1)^2}}\right)}{\sqrt{\mathcal{N}^{2n} - 2\mathcal{N}^n\left(z^n-1\right)+\left(z^n+1\right)^2}} + \frac{n}{2}\ln\left(\frac{\mathcal{N}}{z}\right), \quad (36)$$

which consistently has the asymptotic behavior

$$h_n(z,\theta,\widetilde{Q}) = \begin{cases} \mathcal{O}\left(z^0\right), & \text{for } z \ll 1 \\ -\ln z^n + V_n(z,\theta,\widetilde{Q}) + \frac{n^2\widetilde{Q}^2}{2z} + \mathcal{O}\left(z^{-3/2}\right), & \text{for } z \gg 1 \end{cases}, \quad (37)$$

where $V_n(z,\theta,\widetilde{Q})$ may contain terms that decay slower than $z^{-1}$ but vanish upon angular integration. The divergent part can then be extracted by defining

$$f_n(z,\theta,\widetilde{Q}) = h_n(z,\theta,\widetilde{Q}) + \frac{n}{2}\ln\left(z^2+1\right) + \frac{n^2}{2}\frac{\widetilde{Q}^2}{\sqrt{z^2+1}}, \quad (38)$$

such that the expresion for $\Pi(q)$ is finally

$$\begin{aligned}\Pi(q) &= N\frac{g^2|\boldsymbol{q}|^{2/n}}{(2\pi)^2}\int_0^{2\pi}\frac{d\theta}{2\pi}\int_0^{\widetilde{\Lambda}^2} dz\left\{\left(\epsilon_b^{-1} - \ln|\boldsymbol{q}|^2\right) - \frac{n}{2}\ln\left(z^2+1\right) - \frac{n^2}{2}\frac{\widetilde{Q}^2}{\sqrt{z^2+1}} + f_n(z,\theta,\widetilde{Q})\right\} \\ &= N\frac{g^2|\boldsymbol{q}|^{2/n}}{(2\pi)^2}\left[\widetilde{\Lambda}^2\left(\epsilon_b^{-1} - \ln|\boldsymbol{q}|^2\right) - \frac{n}{2}\widetilde{\Lambda}^2\left(\ln\left(\widetilde{\Lambda}^4+1\right) - 2\right) - n\tan^{-1}\left(\widetilde{\Lambda}^2\right) - \frac{n^2}{2}\widetilde{Q}^2\sinh^{-1}\left(\widetilde{\Lambda}^2\right) + F_n(\widetilde{Q},\widetilde{\Lambda})\right],\end{aligned} \quad (39)$$

where $F_n(\widetilde{Q},\widetilde{\Lambda}) = \int_{-\pi}^{\pi}\frac{d\theta}{2\pi}\int_0^{\widetilde{\Lambda}^2} dz f(z,\theta,\widetilde{Q})$ is UV finite, so we only consider the $\mathcal{O}(\Lambda^0)$ contribution given by $F_n(\widetilde{Q},\infty) \equiv \lim_{\widetilde{\Lambda}\to\infty} F(\widetilde{Q},\widetilde{\Lambda})$. Since this integral is analytically intractable, it is necessary to propose an ansatz that fits well to numerical integration. For a general $n$, we propose the ansatz of the form

$$F_n(\widetilde{Q},\infty) = \mathcal{A}_n^{(1)} + \frac{n^2}{2}\widetilde{Q}^2\left(\ln\left(\widetilde{Q}^2 + \mathcal{A}_n^{(2)}\right) + \mathcal{A}_n^{(3)}\right), \quad (40)$$

where $\mathcal{A}_n^{(i)}$, $i = 1, 2, 3$, are real and $n-$dependent.

For $n = 2$ and $n = 3$ we find:

$$F_{n=2}(\widetilde{Q},\infty) = \left(\pi - \frac{\pi^2}{4}\right) + 2\widetilde{Q}^2\left[\ln\left(\widetilde{Q}^2 + \frac{2\pi}{5}\right) - \frac{3}{5}\right], \quad (41)$$

$$F_{n=3}(\widetilde{Q},\infty) = \left(\frac{3\pi}{2} - \frac{2^{4/3}\pi^{5/2}}{9\Gamma\left(\frac{2}{3}\right)\Gamma\left(\frac{5}{6}\right)}\right) + \frac{9}{2}Q^2\left[\ln\left(\widetilde{Q}^2 + \frac{1}{2}\right) + \frac{1}{2}\right], \quad (42)$$

which are compared to numerical results in Fig. 2.

For general $n$, we conjecture that the final result is:

$$\Pi(\boldsymbol{q},\boldsymbol{Q}) = N\frac{g^2}{(2\pi)^2}\left[\Lambda^2\left(\epsilon_b^{-1} - n\ln\Lambda^2\right) - (2\pi)^2\frac{A_n}{N}|\boldsymbol{q}|^{2/n} - \frac{n^2}{2}|\boldsymbol{Q}|^2\left(\ln\frac{\Lambda^2}{|\boldsymbol{Q}|^2} + \mathcal{O}(1)\right) + \mathcal{O}\left(\frac{|\boldsymbol{q}|^{2/n}}{\Lambda^2}\right)\right], \quad (43)$$

where $A_n$ is a damping coefficient that can be found by means of the following limiting cases.

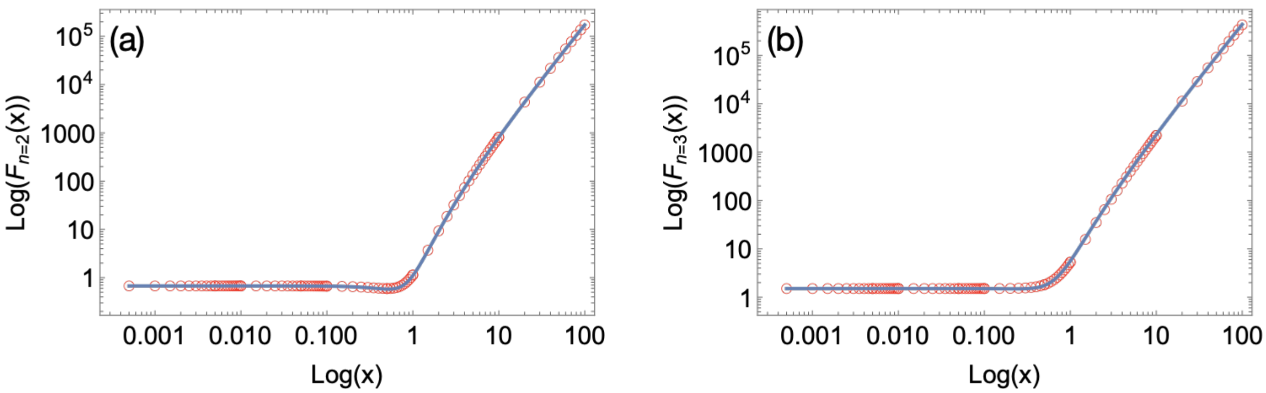


Figure 2: Numerical integration (red markers) of $F_n(\widetilde{Q}, \infty)$ compared to the ansatz (blue line) for (a) $n = 2$ and (b) $n = 3$, given in Eq. (41) and Eq. (42), respectively.

## 2.1 Limiting cases

We recall Eq. (27):

$$\Pi(q) = N\frac{g^2}{\pi}\int_0^1 dx \int \mathrm{d}\boldsymbol{K} \left\{\epsilon_b^{-1} - \ln M + \frac{x(x-1)\boldsymbol{q}^2 + |\boldsymbol{K}|^n|\boldsymbol{K}+\boldsymbol{Q}|^n \cos[n(\phi-\phi')]}{M}\right\}$$

with $M = x(1-x)\boldsymbol{q}^2 + x\left(|\boldsymbol{K}+\boldsymbol{Q}|^n\right)^2 + (1-x)\left(|\boldsymbol{K}|^n\right)^2$.

### (i) $q = 0$:

In this case $M = |\boldsymbol{K}|^{2n}$ and

$$\begin{aligned}\lim_{\boldsymbol{q}\to 0}\lim_{\boldsymbol{Q}\to 0}\Pi(q) &= N\frac{g^2}{\pi}\int_0^1 dx \int \mathrm{d}\boldsymbol{K}\left\{\epsilon_b^{-1} - \ln|\boldsymbol{K}|^{2n} + 1\right\} \\ &= N\frac{g^2\Lambda^2}{(2\pi)^2}\left(\epsilon_b^{-1} - n\ln\Lambda^2\right) \end{aligned} \quad (44)$$

### (ii) $\boldsymbol{Q} = 0$

In this case $M = x(1-x)\boldsymbol{q}^2 + |\boldsymbol{K}|^{2n}$ and

$$\begin{aligned}\lim_{\boldsymbol{Q}\to 0}\Pi(q) &= N\frac{g^2}{\pi}\int_0^1 dx\int \mathrm{d}\boldsymbol{K}\left\{\epsilon_b^{-1} - \ln M + \frac{x(x-1)\boldsymbol{q}^2 + |\boldsymbol{K}|^{2n}}{M}\right\} \\ &= N\frac{g^2}{\pi}\int \mathrm{d}\boldsymbol{K}\left\{\epsilon_b^{-1} - x\ln M\Big|_0^1 + \int_0^1 dx\frac{x(1-2x)\boldsymbol{q}^2 + x(x-1)\boldsymbol{q}^2 + |\boldsymbol{K}|^{2n}}{M}\right\} \\ &= N\frac{g^2|\boldsymbol{q}|^{2/n}}{(2\pi)^2}\int_0^{2\pi}\frac{d\theta}{2\pi}\int_0^{\widetilde{\Lambda}^2} dz\left\{\epsilon_b^{-1} - \ln|\boldsymbol{q}|^2 - \ln z^n + \int_0^1 dx\frac{x^2 - z^n}{x(x-1) - z^n}\right\} \\ &= N\left[\frac{g^2\Lambda^2}{(2\pi)^2}\left(\epsilon_b^{-1} - n\ln\Lambda^2\right) - A_n g^2|\boldsymbol{q}|^{2/n}\right] \end{aligned} \quad (45)$$

where

$$A_n = -\frac{1}{(2\pi)^2}\int_0^\infty dz\int_0^1 dx\frac{x^2 - z^n}{x(x-1) - z^n}, \quad (46)$$

which is in agreement with Eq. (41) and Eq. (42), where for $n = 2$ and $n = 3$, we find, respectively

$$A_2 = \frac{1}{16}, \ A_3 = \frac{2^{-2/3}\pi^{1/2}}{9\Gamma\left(\frac{2}{3}\right)\Gamma\left(\frac{5}{6}\right)}, \ A_4 = \frac{\Gamma[\frac{5}{4}]^2}{\sqrt{2}\,\pi^{3/2}}. \tag{47}$$

Notice that $A_n$ is defined in the sense of the principal value.

**(iii)** $\boldsymbol{q} = 0$

In this case $M = x\left(|\boldsymbol{K}+\boldsymbol{Q}|^n\right)^2 + (1-x)\left(|\boldsymbol{K}|^n\right)^2$ and it is convenient to scale out $\boldsymbol{Q}$ with $|\boldsymbol{K}| = |\boldsymbol{Q}|\sqrt{z}$, $\Lambda = \widetilde{\Lambda}|\boldsymbol{Q}|$:

$$M = |\boldsymbol{Q}|^{2n}[x(1+z+2\sqrt{z}\cos\theta)^3 + (1-x)z^3]$$

defining $\mathcal{N} = 1 + z + 2\sqrt{z}\cos\theta$:

$$\begin{aligned}
\lim_{\boldsymbol{q}\to 0}\Pi(q) &= N\frac{g^2|\boldsymbol{Q}|^2}{(2\pi)^2}\int_0^{2\pi}\frac{d\theta}{2\pi}\int_0^{\widetilde{\Lambda}^2} dz\left\{\epsilon_b^{-1} - x\ln M\Big|_0^1 + \int_0^1 dx\frac{x\left(\mathcal{N}^n - z^n\right) + z^n + P_n(z,\theta,\widetilde{Q})}{x\mathcal{N}^n + (1-x)z^n}\right\} \\
&= N\frac{g^2|\boldsymbol{Q}|^2}{(2\pi)^2}\int_0^{2\pi}\frac{d\theta}{2\pi}\int_0^{\widetilde{\Lambda}^2} dz\left\{\epsilon_b^{-1} - \ln|\boldsymbol{Q}|^{2n} - \ln\mathcal{N}^n + 1 + \int_0^1 dx\frac{P_n(z,\theta,\widetilde{Q})}{x\mathcal{N}^n + (1-x)z^n}\right\} \\
&= N\frac{g^2|\boldsymbol{Q}|^2}{(2\pi)^2}\int_0^{2\pi}\frac{d\theta}{2\pi}\int_0^{\widetilde{\Lambda}^2} dz\left\{\epsilon_b^{-1} - \ln|\boldsymbol{Q}|^{2n} - \ln z^n - \frac{n^2/2}{\sqrt{1+z^2}} + f(z,\theta)\right\} \\
&= N\frac{g^2|\boldsymbol{Q}|^2}{(2\pi)^2}\left[\widetilde{\Lambda}^2(\epsilon_b^{-1} - \ln|\boldsymbol{Q}|^{2n}) - \frac{n^2}{2}\sinh^{-1}(\widetilde{\Lambda}^2) - n\widetilde{\Lambda}^2\ln\widetilde{\Lambda}^2 + \mathcal{O}(1)\right] \\
&= N\frac{g^2\Lambda^2}{(2\pi)^2}\left(\epsilon_b^{-1} - n\ln\Lambda^2\right) - N\frac{g^2|\boldsymbol{Q}|^2}{(2\pi)^2}\left[\frac{n^2}{2}\ln\frac{\Lambda^2}{|\boldsymbol{Q}|^2} + \mathcal{O}(1)\right]
\end{aligned} \tag{48}$$

where we have used that $f(z,\theta)$ decays faster than $z^{-1}$.

# 3 Derivation of the RG equations

Defining $\Gamma_{ij} = \sigma_i \otimes \sigma_j$, we first rewrite the inverse fermionic propagator from Eq. (12) as

$$G_0^{-1}(k) = ik_0 + H_n(k_x,k_y,k_z) = i\ \Gamma_{13}\left[\boldsymbol{k}\cdot\boldsymbol{\gamma} + |\boldsymbol{K}|^n\hat{\boldsymbol{n}}_{\boldsymbol{k}}\cdot\boldsymbol{\Gamma}\right], \tag{49}$$

where $\boldsymbol{\gamma} = (\Gamma_{13}, -\Gamma_{20})$, $\boldsymbol{\Gamma} = (\Gamma_{12}, -\Gamma_{11})$ and $\hat{\boldsymbol{n}}_{\boldsymbol{k}} = (\cos(n\phi),\ \sin(n\phi))$, with $\phi \equiv \phi_{\boldsymbol{k}}$.

At an intermediate momentum scale $\mu$, the action in Eq. (2) takes the form

$$S = i\sum_{n=1}^{N_f}\int_k \psi_{n,k}^{\dagger}\Gamma_{13}\left[\boldsymbol{k}\cdot\boldsymbol{\gamma} + |\boldsymbol{K}|^n\hat{n}_k\cdot\boldsymbol{\Gamma}\right]\psi_{n,k} + \frac{1}{8}\int_q\left(|\boldsymbol{Q}|^2 + M^2\right)\mathrm{tr}\left\{\widetilde{\Phi}_{-q}\widetilde{\Phi}_q\right\} + \frac{g\mu^{(3-d)/2}}{\sqrt{N_f}}\sum_{n=1}^{N_f}\int_{k,q}\bar{\psi}_{n,k+q}\widetilde{\Phi}_q\psi_{n,k}, \tag{50}$$

where $g \equiv g_0\mu^{(d-3)/2}$ is the dimensionless Yukawa coupling and $\widetilde{\Phi}_q = \phi_1(q)\Upsilon_1 + \phi_2(q)\Upsilon_2$. Since all the terms are renormalizable, by adding the corresponding counterterms and setting the renormalized bosonic mass $M$ to zero we get the renormalized action

$$S_r = i\int_k \psi_k^{\dagger}\left[\mathcal{Z}_1\boldsymbol{k}\cdot\boldsymbol{\gamma} + \mathcal{Z}_2|\boldsymbol{K}|^n\hat{n}_k\cdot\boldsymbol{\Gamma}\right]\psi_k + \frac{1}{8}\int_q \mathcal{Z}_3|\boldsymbol{Q}|^2\,\mathrm{tr}\left\{\widetilde{\Phi}_{-q}\widetilde{\Phi}_q\right\} + g\mu^{(3-d)/2}\mathcal{Z}_4\int_{k,q}\bar{\psi}_{k+q}\widetilde{\Phi}_q\psi_k, \tag{51}$$

where $\mathcal{Z}_n = 1 + Z_n/\epsilon$. The relations between the bare and renormalized quantities are

$$\boldsymbol{k}_B = \mathcal{Z}_{\boldsymbol{k}}^{-1}\boldsymbol{k}, \qquad \boldsymbol{K}_B = \boldsymbol{K}, \qquad \psi_B = \sqrt{\mathcal{Z}_\psi}\psi, \qquad \phi_B = \sqrt{\mathcal{Z}_\phi}\phi, \qquad g_B = \mu^{\frac{3-d}{2}}\frac{\mathcal{Z}_{\boldsymbol{k}}^4\mathcal{Z}_4}{\mathcal{Z}_\psi\sqrt{\mathcal{Z}_\phi}}g, \tag{52}$$

where $\mathcal{Z}_{\boldsymbol{k}} = \mathcal{Z}_2/\mathcal{Z}_1$, $\mathcal{Z}_\psi = \mathcal{Z}_2\mathcal{Z}_{\boldsymbol{k}}^2$ and $\mathcal{Z}_\phi = \mathcal{Z}_3\mathcal{Z}_{\boldsymbol{k}}^2$. The anisotropy exponent $z_{\boldsymbol{k}}$ and the anomalous dimensions of the fields are defined as

$$z_{\boldsymbol{k}} = n - \frac{\partial \ln \mathcal{Z}_{\boldsymbol{k}}}{\partial \ln \mu}, \qquad \eta_\psi = \frac{1}{2}\frac{\partial \ln \mathcal{Z}_\psi}{\partial \ln \mu}, \qquad \eta_\phi = \frac{1}{2}\frac{\partial \ln \mathcal{Z}_\phi}{\partial \ln \mu}, \tag{53}$$

while the beta function for $g$ in terms of the momentum scale $\mu$ is obtained from $\frac{\partial g_B}{\partial \ln \mu} = 0$. This leads to a set of coupled equations

$$\mathcal{Z}_1\mathcal{Z}_2\,(z_{\boldsymbol{k}} - n) + (\mathcal{Z}_1\partial_g\mathcal{Z}_2 - \mathcal{Z}_2\partial_g\mathcal{Z}_1)\,\beta_g = 0, \tag{54}$$

$$2\mathcal{Z}_2\,[\eta_\psi + (z_{\boldsymbol{k}} - n)] - \beta_g\partial_g\mathcal{Z}_2 = 0, \tag{55}$$

$$2\mathcal{Z}_3\,[\eta_\phi + (z_{\boldsymbol{k}} - n)] - \beta_g\partial_g\mathcal{Z}_3 = 0, \tag{56}$$

$$(g\partial_g\mathcal{Z}_4 + \mathcal{Z}_4)\,\beta_g + g\mathcal{Z}_4\,[(3-d)/2 - 4\,(z_{\boldsymbol{k}} - n) - 2\eta_\psi - \eta_\phi] = 0, \tag{57}$$

where $\beta_g = \frac{\partial g}{\partial \ln \mu}$. We set $d = 3 - \epsilon$, and solve this equations to obtain

$$z_{\boldsymbol{k}} = n - \frac{1}{2}g\partial_g\,(Z_1 - Z_2)\,, \tag{58}$$

$$\eta_\psi = -\frac{1}{4}g\partial_g Z_2 - (z_{\boldsymbol{k}} - n)\,, \tag{59}$$

$$\eta_\phi = -\frac{1}{4}g\partial_g Z_3 - (z_{\boldsymbol{k}} - n)\,, \tag{60}$$

$$\beta_g = g\left[-\frac{\epsilon}{2} + 4\,(z_{\boldsymbol{k}} - n) + 2\eta_\psi + \eta_\phi\right] + \frac{1}{2}g^2\partial_g Z_4. \tag{61}$$

# 4 One-loop counter-terms

## 4.1 Boson self-energy

We first extract the divergent coefficient of $|\boldsymbol{Q}|^2$ in the polarization insertion by making the replacement $\ln\Lambda^2 \to 2/\epsilon$ in Eq. (48). Consequently, we conjecture that

$$\Pi(\boldsymbol{Q}) - \Pi(0) = -N\frac{n^2g^2}{(2\pi)^2\epsilon}|\boldsymbol{Q}|^2.$$

Therefore, we find

$$Z_3 = -N\frac{n^2g^2}{(2\pi)^2}. \tag{62}$$

## 4.2 Fermion self-energy

Here we consider the sunrise correction with the dressed boson propagator $D^{-1}(q) = N(A_n g^2|\boldsymbol{q}|^{2/n} + |\boldsymbol{Q}|^2)$. We write the bare fermion propagator as $\mathcal{G}_0(k) \equiv G_0(k)\Gamma_{13}$.

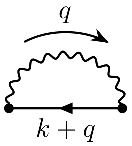


$$= i\ \Sigma(k) = i\frac{N_b g^2}{N_f}\int dq\ \mathcal{G}_0(k+q)D(q) = \frac{N_b g^2}{N N_f}\int dq \frac{(\boldsymbol{k}+\boldsymbol{q})\cdot\boldsymbol{\gamma} + |\boldsymbol{K}+\boldsymbol{Q}|^n \hat{n}_{k+q}\cdot\boldsymbol{\Gamma}}{|\boldsymbol{k}+\boldsymbol{q}|^2 + |\boldsymbol{K}+\boldsymbol{Q}|^{2n}}\frac{1}{A_n g^2|\boldsymbol{q}|^{2/n} + |\boldsymbol{Q}|^2}. \tag{63}$$

## (i) $\boldsymbol{K} = 0$:

We define $\hat{k}\cdot\hat{q} = \cos\theta_q$ as the independent angle for integration and scale $|\boldsymbol{q}| \mapsto |\boldsymbol{Q}|^n y$. Defining $x = |\boldsymbol{k}|/|\boldsymbol{Q}|^n$ and retaining only the leading order in $A_n g^2$:

$$\begin{aligned}
i\ \Sigma(\boldsymbol{k}) &= \frac{N_b g^2}{N N_f}\int dq \frac{(\boldsymbol{k}+\boldsymbol{q})\cdot\boldsymbol{\gamma} + |\boldsymbol{Q}|^n \hat{n}_q\cdot\boldsymbol{\Gamma}}{|\boldsymbol{k}+\boldsymbol{q}|^2 + |\boldsymbol{Q}|^{2n}}\frac{1}{A_n g^2|\boldsymbol{q}|^{2/n} + |\boldsymbol{Q}|^2} \\
&= \frac{N_b g^2}{N N_f}\int \mathrm{d}\boldsymbol{Q}|\boldsymbol{Q}|^{n-2}\int_0^\infty \frac{dy}{2\pi}\frac{y}{(A_n g^2)\, y^{2/n}+1}\int_0^{2\pi}\frac{d\theta_q}{2\pi}\frac{\left(y\cos\theta_q + \frac{|\boldsymbol{k}|}{|\boldsymbol{Q}|^n}\right)\hat{k}\cdot\boldsymbol{\gamma} + y\,\cancel{\sin\theta_q}\,\hat{k}_\perp\cdot\boldsymbol{\gamma} + \hat{n}_q\cdot\boldsymbol{\Gamma}}{y^2 + \left(\frac{|\boldsymbol{k}|}{|\boldsymbol{Q}|^n}\right)^2 + 1 + 2y\frac{|\boldsymbol{k}|}{|\boldsymbol{Q}|^n}\cos\theta_q} \\
&= \frac{N_b g^2}{N N_f}\int \mathrm{d}\boldsymbol{Q}|\boldsymbol{Q}|^{n-2}\int_0^\infty \frac{dy}{2\pi}y\left[\frac{\left(x^2 + \sqrt{x^4 - 2x^2(y^2-1) + (y^2+1)^2} - y^2 - 1\right)\hat{k}\cdot\boldsymbol{\gamma} + 2x\ \hat{n}_q\cdot\boldsymbol{\Gamma}}{2x\sqrt{(x^2+y^2+1)^2 - 4x^2y^2}}\right] + \mathcal{O}(A_n g^2) \\
&= \frac{N_b g^2}{N N_f}\int \mathrm{d}\boldsymbol{Q}|\boldsymbol{Q}|^{n-2}\int_0^\infty \frac{dy}{2\pi}y\left[\frac{\cancel{\hat{n}_q\cdot\boldsymbol{\Gamma}}}{y^2+1} + \frac{x\hat{k}\cdot\boldsymbol{\gamma}}{(y^2+1)^2} + \mathcal{O}(x^2)\right] \\
&= \frac{N_b g^2}{N N_f}\frac{1}{4\pi}\int \mathrm{d}\boldsymbol{Q}\frac{\boldsymbol{k}\cdot\boldsymbol{\gamma}}{|\boldsymbol{Q}|^2}\underbrace{\int_0^\infty \frac{dy}{2\pi}\frac{y}{(1+y^2)^2}}_{1/4\pi} \\
&\approx \frac{N_b g^2}{(4\pi)^2 N N_f}\frac{2}{\epsilon}\boldsymbol{k}\cdot\boldsymbol{\gamma}.
\end{aligned} \tag{64}$$

Therefore, we obtain

$$Z_1 = -\frac{N_b g^2}{2(2\pi)^2 N N_f}. \tag{65}$$

## (ii) $\boldsymbol{k} = 0$:

Here we scale $|\boldsymbol{q}| \mapsto |\boldsymbol{Q}|^n (Ag^2)^{-n/2} y$:

$$
\begin{aligned}
i\ \Sigma(\boldsymbol{K}) &= \frac{N_b g^2}{N N_f}\int \mathrm{d}q \frac{\cancel{\boldsymbol{q}\cdot\boldsymbol{\gamma}} + |\boldsymbol{K}+\boldsymbol{Q}|^n \hat{n}_{k+q}\cdot\boldsymbol{\Gamma}}{|\boldsymbol{q}|^2 + |\boldsymbol{K}+\boldsymbol{Q}|^{2n}} \frac{1}{A_n g^2 |\boldsymbol{q}|^{2/n} + |\boldsymbol{Q}|^2} \\
&= \frac{N_b g^2}{N N_f}\int \frac{\mathrm{d}\boldsymbol{Q}}{|\boldsymbol{Q}|^2}\int_0^\infty \frac{dy}{2\pi}\frac{y}{y^{2/n}+1}\frac{|\boldsymbol{K}+\boldsymbol{Q}|^n \hat{n}_{k+q}\cdot\boldsymbol{\Gamma}}{y^2 + \left(\frac{A_n g^2 |\boldsymbol{K}+\boldsymbol{Q}|^2}{|\boldsymbol{Q}|^2}\right)^n} \\
&= \frac{N_b g^2}{4\pi N N_f}\int \mathrm{d}\boldsymbol{Q}\frac{|\boldsymbol{K}+\boldsymbol{Q}|^n \hat{n}_{k+q}\cdot\boldsymbol{\Gamma}}{(A_n g^2)^n\,|\boldsymbol{K}+\boldsymbol{Q}|^{2n} - |\boldsymbol{Q}|^{2n}}\left(n|\boldsymbol{Q}|^{2n-2}\ln\frac{(A_n g^2)|\boldsymbol{Q}+\boldsymbol{K}|^2}{|\boldsymbol{Q}|^2} + \mathcal{O}(A_n g^2)\right) \\
&= \frac{N_b g^2}{4\pi N N_f} n\int \mathrm{d}\boldsymbol{Q}\frac{|\boldsymbol{K}+\boldsymbol{Q}|^n \hat{n}_{k+q}\cdot\boldsymbol{\Gamma}}{|\boldsymbol{Q}|^2}\left(\ln\frac{1}{A_n g^2} + \ln\frac{|\boldsymbol{Q}|^2}{|\boldsymbol{K}+\boldsymbol{Q}|^2}\right) + \mathcal{O}(Ag^2) \\
&= \frac{N_b g^2}{4\pi N N_f} n(I_1 + I_2).
\end{aligned}
\tag{66}
$$

At this point it is convinient to write the numerator in cartesian coordinates and exploit the simplifications allowed by symmetry when integrating over $\boldsymbol{Q}$. We conjecture that

$$
I_1 = \ln\frac{1}{A_n g^2}\int \mathrm{d}\boldsymbol{Q}\frac{|\boldsymbol{K}+\boldsymbol{Q}|^n \hat{n}_{k+q}\cdot\boldsymbol{\Gamma}}{|\boldsymbol{Q}|^2} = \ln\frac{1}{A_n g^2}\int \mathrm{d}\boldsymbol{Q}\frac{|\boldsymbol{K}|^n \hat{n}_k\cdot\boldsymbol{\Gamma}}{|\boldsymbol{Q}|^2} \approx \ln\frac{1}{A_n g^2}\frac{1}{4\pi}\frac{2}{\epsilon}|\boldsymbol{K}|^n \hat{n}_k\cdot\boldsymbol{\Gamma}. \tag{67}
$$

Using the relation $\ln\big(1+a^{-1}\big) = \int_0^1 dx(x+a)^{-1}$ we can perform the second integral. We conjecture:

$$
\begin{aligned}
I_2 &= -\int \mathrm{d}\boldsymbol{Q}\frac{|\boldsymbol{K}+\boldsymbol{Q}|^n \hat{n}_{k+q}\cdot\boldsymbol{\Gamma}}{|\boldsymbol{Q}|^2}\ln\frac{|\boldsymbol{K}+\boldsymbol{Q}|^2}{|\boldsymbol{Q}|^2} \\
&= -\int \mathrm{d}\boldsymbol{Q}\frac{|\boldsymbol{K}+\boldsymbol{Q}|^n \hat{n}_{k+q}\cdot\boldsymbol{\Gamma}}{|\boldsymbol{Q}|^2}\ln\left(1 + \frac{2\boldsymbol{Q}\cdot\boldsymbol{K} + |\boldsymbol{K}|^2}{|\boldsymbol{Q}|^2}\right) \\
&= -\int \mathrm{d}\boldsymbol{Q}\int_0^1 dx\frac{|\boldsymbol{K}+\boldsymbol{Q}|^n \hat{n}_{k+q}\cdot\boldsymbol{\Gamma}}{|\boldsymbol{Q}|^2}\frac{2\boldsymbol{Q}\cdot\boldsymbol{K} + |\boldsymbol{K}|^2}{x(2\boldsymbol{Q}\cdot\boldsymbol{K} + |\boldsymbol{K}|^2) + |\boldsymbol{Q}|^2} \\
&= -|\boldsymbol{K}|^n \hat{n}_k\cdot\boldsymbol{\Gamma}\int_0^1 dx\int_0^1 dz\ n(1-xz)^{n-1}\int \mathrm{d}\boldsymbol{Q'}\frac{|\boldsymbol{Q'}|^2 + \mathcal{O}(Q'^0)}{(|\boldsymbol{Q'}|^2+\Delta)^2} \\
&= -|\boldsymbol{K}|^n \hat{n}_k\cdot\boldsymbol{\Gamma}\int_0^1 dx\int_0^1 dz\ n(1-xz)^{n-1}\left(\frac{2}{\epsilon} + \text{finite}\right) \\
&\approx -B_n\frac{1}{4\pi}\frac{2}{\epsilon}|\boldsymbol{K}|^n \hat{n}_k\cdot\boldsymbol{\Gamma},
\end{aligned}
\tag{68}
$$

where

$$
B_n = \frac{1}{n} + \sum_{k=1}^{n-1}\frac{1}{k}. \tag{69}
$$

Finally, we obtain

$$
i\ \Sigma(\boldsymbol{K}) = \frac{N_b g^2}{N N_f} n\frac{|\boldsymbol{K}|^n \hat{n}_k\cdot\boldsymbol{\Gamma}}{2(2\pi)^2\epsilon}\left(\ln\frac{1}{A_n g^2} - B_n\right). \tag{70}
$$

Therefore,

$$
Z_2 = -\frac{n g^2 N_b}{2(2\pi)^2 N N_f}\left(\ln\frac{1}{A_n g^2} - B_n\right), \tag{71}
$$

which can be compactly written as

$$
Z_2 = \frac{n g^2 N_b}{2(2\pi)^2 N N_f}\ln\big(C_n g^2\big), \tag{72}
$$

where $C_n = A_n e^{B_n}$.

### 4.3 Vertex correction

Finally, using the anticommutation relations $\{\Gamma_\mu, \Gamma_\nu\} = 2\delta_{\mu\nu}$, we find that the vertex correction takes the form

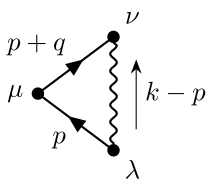


$$= \frac{g^2}{N_f}(N_b - 2)\Gamma_\mu W(k,q). \tag{73}$$

where

$$W(k,q) = \int \mathrm{d}p\ D(k-p)\mathcal{G}_0(p+q)\mathcal{G}_0(p). \tag{74}$$

Since we are after the UV divergent piece with zero momentum transfer, we evaluate

$$W(0,\boldsymbol{Q}) = \frac{(-i)^2}{N}\int \mathrm{d}p \frac{1}{A_n g^2|\boldsymbol{p}|^{2/n} + |\boldsymbol{P}|^2} \frac{\boldsymbol{p}\cdot\boldsymbol{\gamma} + |\boldsymbol{P}+\boldsymbol{Q}|^n(\hat{n}_{p+q}\cdot\boldsymbol{\Gamma})}{|\boldsymbol{p}|^2 + |\boldsymbol{P}+\boldsymbol{Q}|^{2n}} \frac{\boldsymbol{p}\cdot\boldsymbol{\gamma} + |\boldsymbol{P}|^n(\hat{n}_p\cdot\boldsymbol{\Gamma})}{|\boldsymbol{p}|^2 + |\boldsymbol{P}|^{2n}}. \tag{75}$$

In analogy with the fermion self-energy calculation we scale $|\boldsymbol{q}| \mapsto |\boldsymbol{Q}|^n(A_n g^2)^{-n/2}y$, and by inspection we find:

$$\begin{aligned} W(0,\boldsymbol{Q}) &= -\frac{1}{N}\int \frac{\mathrm{d}\boldsymbol{P}}{|\boldsymbol{P}|^2}\int_0^\infty \frac{dy}{2\pi}\frac{y}{y^{2/n}+1}\frac{y^2 + \left(A_n g^2\right)^n \cos\left[n\left(\phi_{p+q}-\phi_p\right)\right]|\boldsymbol{P}+\boldsymbol{Q}|^n/|\boldsymbol{P}|^n}{\left[y^2 + \left(A_n g^2 \frac{|\boldsymbol{P}+\boldsymbol{Q}|^2}{|\boldsymbol{P}|^2}\right)^n\right]\left[y^2 + (A_n g^2)^2\right]} \\ &= \frac{n}{4\pi N}\int \frac{\mathrm{d}\boldsymbol{P}}{|\boldsymbol{P}|^2}\left\{\ln\left(A_n g^2\right) + \frac{|\boldsymbol{P}+\boldsymbol{Q}|^{2n} - |\boldsymbol{P}|^n|\boldsymbol{P}+\boldsymbol{Q}|^n\cos\left[n\left(\phi_{p+q}-\phi_p\right)\right]}{|\boldsymbol{P}+\boldsymbol{Q}|^{2n} - |\boldsymbol{P}|^{2n}}\ln\frac{|\boldsymbol{P}+\boldsymbol{Q}|^2}{|\boldsymbol{P}|^2} + \mathcal{O}(A_n g^2)\right\} \\ &\approx \frac{n}{2(2\pi)^2 N}\ln\left(A_n g^2\right)\frac{1}{\epsilon} + \mathcal{O}(A_n g^2). \end{aligned} \tag{76}$$

Therefore, we find

$$Z_4 = \frac{(N_b-2)}{N N_f}\frac{n g^2}{2(2\pi)^2}\ln\left(A_n g^2\right). \tag{77}$$

## 5 RG fixed points and critical exponents

In this section we evaluate the equations derived in Sec. 3 to find the values for the fixed points ($g_*^2$), anomalous dimensions ($z_{\boldsymbol{k}}, \eta_\psi, \eta_\phi$) and correlation length exponent $\nu$. The RG flow equation given by Eq. (61) with $\ell \equiv -\ln\mu$ is:

$$\frac{dg}{d\ell} = \frac{\epsilon}{2}g - \frac{g^3}{8\pi^2}\left[N n^2 + \frac{N_b + n(N_b-2)}{N N_f} + \frac{n(N_b-2)}{N N_f}\ln\left(A_n g^2\right)\right], \tag{78}$$

with $A_n$ defined in Eq. (46).

At $\epsilon = 0$ and for $N_b \neq 2$, the right-hand vanishes when $g$ takes the value

$$g_*^2 = \frac{1}{A_n}\exp\left[-\frac{N N_f}{n(N_b-2)}\left(N n^2 + \frac{N_b + n(N_b-2)}{N N_f}\right)\right], \tag{79}$$

which implies that the non-interacting fixed point $g_* = 0$ is stable for $N_b = 1$ and 2, but it becomes unstable to an interacting fixed point for $N_b \geq 3$.

At $\epsilon > 0$ ($d_M < 2$), for $N_b \neq 2$ we obtain stable IR fixed points given by

$$g_*^2 = \frac{a}{W_s(a A_n e^b)}, \quad a = \frac{4\pi^2 N N_f \epsilon}{n(N_b-2)}, \quad b = 1 + \frac{N^2 n^2 N_f + N_b}{n(N_b-2)}, \tag{80}$$

where $W_s(x)$ is the product logarithm function on the $s^{\text{th}}$ branch. For $N_b = 1$, $a$ becomes negative, implying that the correct solution is given by $s = -1$. For $N_b \geq 3$ the solutions are given by $s = 0$.

For $N_b = 2$ we find, in the limit $\epsilon \ll 1, N_f \gg 1$:

$$g_*^2 = \frac{4\pi^2}{Nn^2}\left(1 - \frac{2}{N^2 n^2 N_f}\right)\epsilon, \tag{81}$$

$$z_{\boldsymbol{k}} = n + \frac{1}{N^2 n N_f}\epsilon \ln \epsilon, \quad \eta_\psi = -\frac{3}{2N^2 n N_f}\epsilon \ln \epsilon, \quad \eta_\phi = \frac{\epsilon}{2} - \frac{1}{N^2 n N_f}\epsilon \ln \epsilon, \tag{82}$$

$$\nu^{-1} \equiv 2 - 2\eta_\phi = 2 - \epsilon + \frac{2}{N^2 n N_f}\epsilon \ln \epsilon. \tag{83}$$

For $N_b = 3$ we look for a solution of the form $g^2 = g_0^2 B^{1/N_f}$, with $g_0 \sim \epsilon$ and $B$ being $N_f$-independent, to find, to the leading order in $\epsilon$ and $1/N_f$,

$$g_*^2 = \frac{4\pi^2}{Nn^2}\left(e^{1+3/n} A_n \frac{4\pi^2}{Nn^2}\right)^{-1/(N^2 n^2 N_f)} \epsilon^{1-1/(N^2 n^2 N_f)}, \tag{84}$$

$$z_{\boldsymbol{k}} = n + \frac{3n}{2NN_f}\epsilon \ln \epsilon, \quad \eta_\psi = -\frac{9n}{4NN_f}\epsilon \ln \epsilon, \quad \eta_\phi = \frac{Nn^2}{2}\epsilon - \frac{2n}{NN_f}\epsilon \ln \epsilon, \tag{85}$$

$$\nu^{-1} \equiv 2 - 2\eta_\phi = 2 - Nn^2\epsilon + \frac{2n}{NN_f}\epsilon \ln \epsilon. \tag{86}$$

# References

[1] S. Sur and B. Roy, Unifying interacting nodal semimetals: a new route to strong coupling, Phys. Rev. Lett. **123**, 207601 (2019).

[2] B. Roy, P. Goswami, and V. Juricic, Interacting weyl fermions: phases, phase transitions, and global phase diagram, Phys. Rev. B **95**, 201102 (2017).

[3] M. Peskin and D. Schroeder, *An introduction to quantum field theory* (CRC Press, London, England, 2019).
